# Supplementary material for: Revenue Maximization for Selling Multiple Correlated Items
Source: arXiv:1412.3187 source file (2015-07-22)
Supplement: Supplementary file 1 [file core_decomposition_appendix.tex]

\section{Omitted proofs of Section \ref{core-dep}}
